# Supplementary material for: SPI-GAN: Denoising Diffusion GANs with Straight-Path Interpolations
Source: arXiv:2206.14464 source file (2024-03-14)
Supplement: Supplementary file 1 [file 6_appendix.tex]

\section*{Appendix}
\section{Stochastic differential equation (SDE)}\label{a:SDE}
In~\citep{song2020score}, three types of SDE diffusion processes are presented. Depending on the type, $f(\mathbf{x}, t)$ and $g(t)$ are defined as follows: 
\begin{align}
    f(\mathbf{x}, t)&=\begin{cases}0,  &\textrm{ if VE-SDE,}\\
    -\frac{1}{2}\beta(t)\mathbf{x},&\textrm{ if VP-SDE,}\\
    -\frac{1}{2}\beta(t)\mathbf{x},&\textrm{ if sub-VP-SDE,}\\
    \end{cases}\label{eq:drift}\\
    g(t)&=\begin{cases}\sqrt{\frac{\texttt{d}[{\sigma}^2(t)]}{\texttt{d}t}},&\textrm{ if VE-SDE,}\\
    \sqrt{\beta(t)},&\textrm{ if VP-SDE,}\\
    \sqrt{\beta(t)(1-e^{-2\int_0^t \beta(s)\, \texttt{d}s})},&\textrm{ if sub-VP-SDE,}\\
    \end{cases}\label{eq:diffusion_f_g}
\end{align}where ${\sigma}^2(t)$ and $\beta(t)$ are functions w.r.t. time $t$. Full derivatives of VE, VP and sub-VP SDE are presented in~\cite[Appendix. B]{song2020score}.

\section{Effectiveness of the straight-path interpolation}\label{a:effectiveness}
Between $\mathbf{x}_{T}$ and $\mathbf{x}_{0}$, our straight-path interpolation provides a much simpler path than that of the SDE path because it follows the linear equation in Eq.~\eqref{eq:interpolation}. Also, because of the nature of the linear interpolation, its training is robust, even when $\mathbf{i}(u+\Delta u)$ is missing, if $\mathbf{i}(u)$ and $\mathbf{i}(u+2\Delta u)$ are considered. This is not guaranteed if a path from $\mathbf{x}_{T}$ to $\mathbf{x}_{0}$ is non-linear. As a result, SPI-GAN using the straight-path interpolation shows better performance.

One can also derive the following ordinary differential equation (ODE) from the straight-path interpolation definition in Eq.~\eqref{eq:interpolation} after taking the derivative w.r.t. $u$:
\begin{align}\label{eq:spiode}
    \frac{d\mathbf{i}(u)}{du} = \mathbf{x}_0 - \mathbf{x}_T,
\end{align} where one can get $\mathbf{i}(u + h)  = \mathbf{i}(u) + h\frac{d\mathbf{i}(u)}{du} = (u+h)\mathbf{x}_0 + (1-u-h)\mathbf{x}_T$ with the Euler method. In comparison with the SDE in Eqs.~\eqref{eq:drift} and~\eqref{eq:diffusion_f_g}, the ODE provides a much simpler process.

\section{SPI-GAN details}
\label{a:spigan_detail}

In this section, we refer to the detailed model architecture, object function, and training algorithm of our proposed SPI-GAN.

\subsection{Model architecture}
\label{a:model}
The network architectures of StyleGAN2 are modified to implement our proposed straight-path interpolation after adding the NODE-based mapping network and customizing some parts.

\paragraph{Mapping network.}
Our mapping network consists of two parts. First, the network architecture to define the function $\mathbf{o}$ is in Table~\ref{tbl:mapping_o}. Second, the NODE-based network has the following ODE function $\mathbf{r}$ in Table~\ref{tbl:mapping_r}.

\begin{table*}[ht]
\begin{minipage}{\textwidth}
\begin{minipage}{0.49\textwidth}
\vspace{1em}
\caption{The architecture of the network $\mathbf{o}$.}\label{tbl:mapping_o}
\vspace{-1em}
\centering
\scriptsize
\begin{center}
\begin{small}
\begin{sc}
\begin{adjustbox}{width=0.9\textwidth}
\begin{tabular}{cccc}\hline
Layer & Design & Input Size & Output Size \\ \hline
1 & LeakyReLU(Linear) & $ C \times H \times W $  & $  \dim(\mathbf{h})$ \\ \hline
\end{tabular}
\end{adjustbox}
\end{sc}
\end{small}
\end{center}
\end{minipage}
\begin{minipage}{0.49\textwidth}
\vspace{1em}
\caption{The architecture of the network $\mathbf{r}$. }\label{tbl:mapping_r}
\vspace{-1em}
\centering
\scriptsize
\begin{center}
\begin{small}
\begin{sc}
\begin{adjustbox}{width=0.9\textwidth}
\begin{tabular}{cccc}\hline
Layer & Design & Input Size & Output Size \\ \hline
1 & LeakyReLU(Linear) & $ \dim(\mathbf{h})$  & $  \dim(\mathbf{h})$ \\ \hline
\end{tabular}
\end{adjustbox}
\end{sc}
\end{small}
\end{center}
\end{minipage}
\end{minipage}
\end{table*}

% \begin{table}[ht]
% \caption{The architecture of the network $\mathbf{o}$.}\label{tbl:mapping_o}
% \begin{minipage}{0.5\columnwidth}
% \centering
% \scriptsize
% \begin{tabular}{cccc}\hline
% Layer & Design & Input Size & Output Size \\ \hline
% 1 & LeakyReLU(Linear) & $ C \times H \times W $  & $  \dim(\mathbf{h})$ \\ \hline
% \end{tabular}
% % \vspace{1 em}
% \end{minipage}
% \caption{The architecture of the network $\mathbf{r}$. }\label{tbl:mapping_r}
% % \vspace{-1 em}
% \begin{minipage}{0.5\columnwidth}
% \centering
% \scriptsize
% \begin{tabular}{cccc}\hline
% Layer & Design & Input Size & Output Size \\ \hline
% 1 & LeakyReLU(Linear) & $ \dim(\mathbf{h})$  & $  \dim(\mathbf{h})$ \\ \hline
% \end{tabular}
% \end{minipage}
% \end{table}

% \begin{table}[ht]
% \caption{The architecture of the network $\mathbf{r}$. }\label{tbl:mapping_r}
% % \vspace{-1 em}
% \begin{minipage}{\columnwidth}
% \centering
% \scriptsize
% \begin{tabular}{cccc}\hline
% Layer & Design & Input Size & Output Size \\ \hline
% 1 & LeakyReLU(Linear) & $ \dim(\mathbf{h})$  & $  \dim(\mathbf{h})$ \\ \hline
% \end{tabular}
% \end{minipage}
% \end{table}

\paragraph{Generator.}
We follow the original StyleGAN2 architecture. However, we use the latent vector $\mathbf{h}(u)$ instead of the intermediate latent code w of StyleGAN2.

\paragraph{Discriminator.} The network architecture of the discriminator is also based on StyleGAN2~\citep{karras2020analyzing} --- StyleGAN2 has two versions for the discriminator, i.e., Original and Residual. However, our discriminator receives time $u$ as a conditional input. To this end, we use the positional embedding of the time value as in~\citep{ho2020denoising}. The hyperparameters for the discriminator are in Table~\ref{tbl:hyper}.

\subsection{Object function}\label{A:trainingdetails}
We train our model using the Adam optimizer for training both the generator and the discriminator. We use the exponential moving average (EMA) when training the generator, which achieves high performance in~\citep{ho2020denoising,song2020score,karras2020training}. The hyperparameters for the optimizer are in Table~\ref{tbl:hyper}. The adversarial training object of our model is as follows:
\begin{align}\begin{split}\label{eq:object}
    & \min_{\phi}  \mathbb{E}_{\mathbf{i}(u) \sim \mathbf{q}_{\mathbf{i}(u)}} \big[-\text{log}(D_{\phi}(\mathbf{i}(u),u))\\ &+\mathbb{E}_{\mathbf{z} \sim \mathcal{N}(\mathbf{0}, \sigma^{2}\mathbf{I})} \big[ -\text{log}(1-D_{\phi}(G_{\theta}(M_{\psi}(\mathbf{z})), u)) \big] \big] ,  \\ & \max_{\theta, \psi} \mathbb{E}_{\mathbf{i}(t) \sim \mathbf{q}_{\mathbf{i}(u)}}\big[\mathbb{E}_{\mathbf{z} \sim \mathcal{N}(\mathbf{0}, \sigma^{2}\mathbf{I})} \big[ \text{log}(D_{\phi}(G_{\theta}(M_{\psi}(\mathbf{z})), u)) \big]\big],
\end{split}\end{align}
where, $\mathbf{q}_{\mathbf{i}(u)}$ is the interpolated image distribution, $D_{\phi}$ is denoted as the discriminator, $G_{\theta}$ is denoted as the generator, and $M_{\psi}$ is denoted as the mapping network of our model. We also use the $R_1$ regularization and the path length regularization~\citep{karras2020analyzing}. $\lambda_{R_1}$ (resp. $\lambda_{path}$) means the coefficient of the $R_1$ regularization term (resp. the coefficient of the path length regularization term). Each regularizer term is as follows:
\begin{align}\label{eq:object2}
    R_1(\phi) =& \lambda_{R_1}\mathbb{E}_{q(\mathbf{i}(u))}\big[ \|\nabla_{\mathbf{i}(t)}(D_{\phi}(\mathbf{i}(u) | u))  \ \|^2\big], \\
    \text{Path length} =& \lambda_{path}\mathbb{E}_{\mathbf{h}(u), \mathbf{i}(u)}\big( \| \textbf{J}^{T}_{\mathbf{h}(u)}\mathbf{i}(u)  \ \|_2 - a \big),
\end{align}where $\textbf{J}_{\mathbf{h}(u)}=\partial G_{\theta}(\mathbf{h}(u))/ \partial \mathbf{h}(u)$ is the Jacobian matrix. The constant $a$ is set dynamically during optimization to find an appropriate global scale. The path length regularization helps with the mapping from latent vectors to images. The lazy regularization makes training stable by computing the regularization terms ($R_1$, path length) less frequently than the main loss function. In SPI-GAN, the regularization term for the generator and the discriminator is calculated once every 4 iterations and once every 16 iterations, respectively. The hyperparameters for the regularizers are in Table~\ref{tbl:hyper}.

\subsection{Training algorithm}\label{a:training_algorithm}
There is a training algorithm. The two main differences with the sampling algorithm are i) we sample a set of noisy vectors $\{\mathbf{z}^l\}_{l=1}^N$ whereas we use $\{\mathbf{x}_T^{l}\}_{l=1}^N$ in the training algorithm, and ii) for sampling, we need only $\{\mathbf{h}^l(1)\}_{l=1}^N$.

\begin{algorithm}[H]
    \caption{How to train SPI-GAN}
    \label{alg:train}
    \textbf{Input}: Training data $D_{\text{train}}$, Maximum iteration numbers $max\_iter$ 
    % \textbf{Parameter}: discriminator $\phi$, mapping network $\psi$, generator $\theta$
    \begin{algorithmic}[1]
    \STATE Initialize discriminator $\phi$, mapping net. $\psi$, generator $\theta$
    \STATE $iter  \gets 0$
    \WHILE{$iter < max\_iter$}
    \STATE Create a mini-batch of real images $\{\mathbf{x}_0^{l}\}_{l=1}^N$, where $\mathbf{x}_0^{l}$ means $l$-th real image
    \STATE Calculate a mini-batch of noisy images $\{\mathbf{x}_T^{l}\}_{l=1}^N$ with the forward SDE path
    \STATE Sample $u$, where $u \in (0,1]$
    \STATE Calculate $\{\mathbf{h}^l(u)\}_{l=1}^N$ with the mapping network which processes $\{\mathbf{x}_T^{l}\}_{l=1}^N$
    \STATE Generate fake images $\{\hat{\mathbf{i}}^l(u)\}_{l=1}^N$ with the generator
    \IF {$iter\mod 2 \equiv 0$}
    \STATE Calculate $\{\mathbf{i}^l(u)\}_{l=1}^N$ with Eq.~\ref{eq:interpolation} 
    \STATE Update $\phi$\ via adversarial training
    \ELSE
    \STATE Update $\psi$ and $\theta$  via adversarial training
    \ENDIF
    \STATE $iter \gets iter + 1$
    \ENDWHILE
    \STATE \textbf{return} $\phi, \psi, \theta$
\end{algorithmic}
\end{algorithm}
\section{Experimental details}
In this section, we describe the detailed experimental environments of SPI-GAN. We build our experiments on top of~\citep{kang2022studiogan}

%~\url{https://github.com/POSTECH-CVLab/PyTorch-StudioGAN}~\citep{kang2022studiogan}.\footnote{The MIT License}

\subsection{Experimental environments}\label{a:detail}
Our software and hardware environments are as follows: \textsc{Ubuntu} 18.04 LTS, \textsc{Python} 3.9.7, \textsc{Pytorch} 1.10.0, \textsc{CUDA} 11.1, \textsc{NVIDIA} Driver 417.22, i9 CPU, \textsc{NVIDIA RTX A5000}, and \textsc{NVIDIA RTX A6000}.

\subsection{Target diffusion model}
\label{a:diffusion}
Our model uses a forward SDE to transform an image ($\mathbf{x}_0$) into a noise vector ($\mathbf{x}_T$). When generating a noise vector, we use the forward equation of VP-SDE for its high efficacy/effectiveness. The $\beta(t)$ function of VP-SDE is as follows:
\begin{align}
    \beta(t) = \beta_{\text{min}} + t(\beta_{\text{max}}-\beta_{\text{min}}),
    %\boldsymbol{\sigma}^2(t') = 1-e^{-\beta_{\text{min}}t'-0.5(\beta_{\text{max}}-\beta_{\text{min}})t'^{2}},
    \label{beta}
\end{align}where $\beta_{\text{max}}$ = 20, $\beta_{\text{min}}$ = 0.1, and $t':= \frac{t}{T}$ which is normalized from $t\in\{0, 1, \dots, T\}$ to $[0,1]$. Under these conditions, \cite[Appendix B]{song2020score} proves that the noise vector at $t'=1$ ($\mathbf{x}_T$) follows a unit Gaussian distribution.

\subsection{Data augmentation} 
Our model uses the adaptive discriminator augmentation (ADA)~\citep{karras2020training}, which has shown good performance in StyleGAN2.\footnote{\url{https://github.com/NVlabs/stylegan2} (Nvidia Source Code License)} The ADA applies image augmentation adaptively to training the discriminator. We can determine the maximum degree of the data augmentation, which is known as an ADA target, and the number of the ADA learning can be determined through the ADA interval. We also apply mixing regularization ($\lambda_{mixing}$) to encourage the styles to localize. Mixing regularization determines how many percent of the generated images are generated from two noisy images during training (a.k.a, style mixing). There are hyperparameters for the data augmentation in Table~\ref{tbl:hyper}.

\subsection{Hyperparameters}
We list all the key hyperparameters in our experiments for each dataset. Our supplementary material accompanies some trained checkpoints and one can easily reproduce.

\begin{table}[h]
\caption{Hyperparameters set for SPI-GAN.}\label{tbl:hyper}
\centering
\begin{adjustbox}{width=0.8\textwidth}
\begin{tabular}{llccc}
\hline
 &  & CIFAR-10 & CelebA-HQ-256 & LSUN-Church-256 \\ \hline
\multirow{3}{*}{Augmentation} & ADA target & 0.6 & 0.6 & 0.6 \\
 & ADA interval & 4 & 4 & 4 \\
 & $\lambda_{mixing}$ ($\%$) & 0 & 90 & 90 \\ \hline
\multirow{2}{*}{Architecture} & Mapping network & 1 & 7 & 7 \\
 & Discriminator & Original & Residual & Residual \\ \hline
\multirow{4}{*}{Optimizer} & Learning rate for generator  & 0.0025 & 0.0025 & 0.0025 \\
 & Learning rate for discriminator & 0.0025 & 0.0025 & 0.0025 \\
 & EMA & 0.999 & 0.999 & 0.999 \\ 
 & ODE Solver & \multicolumn{3}{c}{4th order Runge–Kutta} \\ \hline
\multirow{4}{*}{Regularization} & Lazy generator & 4 & 4 & 4 \\
 & Lazy discriminator & 16 & 16 & 16 \\
 & $\lambda_{R_1}$ & 0.01 & 10 & 10 \\
 & $\lambda_{path}$ & 0 & 2 & 2 \\ \hline
\end{tabular}
\end{adjustbox}
\end{table}
    
% \subsection{Sampling method of SPI-GAN}
% \label{a:sampling}

% \begin{algorithm}[h]
%     \caption{How to sampling SPI-GAN}
%    \label{alg:sampling}
%     \textbf{Input}: Noisy vectors $\mathbf{z}^{l} \sim \mathcal{N}(\mathbf{0}, \sigma^{2}\mathbf{I})$ 
    
%     \begin{algorithmic}[1]
%     \STATE Sample a set of noisy vectors $\{\mathbf{z}^l\}_{l=1}^N$\;
%    \STATE Calculate $\{\mathbf{h}^l(1)\}_{l=1}^N$ via the mapping network which processes $\{\mathbf{z}^l\}_{l=1}^N$ by solving Eq.~\eqref{eq:mapping} after setting $u=1$\;
%    \STATE Generate a fake image $\{\hat{\mathbf{i}}^l(1)\}_{l=1}^N$ with the generator\;
%    \STATE \textbf{return} fake image $\{\hat{\mathbf{i}}^l(1)\}_{l=1}^N$\;
% \end{algorithmic}
% \end{algorithm}

% \clearpage
\section{Visualization}
\label{a:visualization}

We introduce interpolation and several high-resolution generated samples.

\subsection{Interpolation}\label{a:interpolation}

\begin{figure}[h]
\small
% \vspace{1em}
\centering
\begin{minipage}{0.9\linewidth}
\centering
     \includegraphics[width=.5\linewidth]{images/interpolation_latent.png}
     \caption{Generation by interpolating $\mathbf{h}(1) = (1-a)\mathbf{h}(1)' + a \mathbf{h}(1)''$, where $0 \leq a \leq 1$.}
    \label{fig:interpolationlatent}
\end{minipage}\hfill
\end{figure}

% \clearpage
\subsection{CIFAR-10}
% \centering
\begin{figure}[h]
\centering
\includegraphics[width=0.8\columnwidth]{images/cifar10_appendix.png}
\caption{Qualitative results on CIFAR-10.}\label{fig:cifar10_appendix}
\end{figure}

%\clearpage
\subsection{Qualitative results on high resolution datasets}
\begin{figure*}[h]
    \centering
    \begin{minipage}{0.49\linewidth}
        \centering
        \includegraphics[width=\columnwidth]{images/celeba_appendix.png}
\caption{CelebA-HQ-256}\label{fig:celeba_appendix}
    \end{minipage}
    \begin{minipage}{0.49\linewidth}
        \centering
\includegraphics[width=\columnwidth]{images/lsun_appendix.png}
\caption{LSUN-Church-256}\label{fig:lsun_appendix}
    \end{minipage}
\end{figure*}

% \subsection{CelebA-HQ-256}
% \begin{figure}[ht]
% \centering
% \includegraphics[width=0.58\columnwidth]{images/celeba_appendix.png}
% \caption{Qualitative results on CelebA-HQ-256.}\label{fig:celeba_appendix}
% \end{figure}

% \clearpage
% \subsection{LSUN-Church-256}
% \begin{figure}[ht]
% \centering
% \includegraphics[width=0.58\columnwidth]{images/lsun_appendix.png}
% \caption{Qualitative results on LSUN-Church-256.}\label{fig:lsun_appendix}
% \end{figure}

\begin{figure}[t]
\centering
{\includegraphics[width=.50\columnwidth]{images/interpolation.png}
\includegraphics[width=.49\columnwidth]{images/interpolation_real.png}}
\caption{\textbf{Left:} Generation by varying the latent vector from $\mathbf{h}(0)$ to $\mathbf{h}(1)$ given fixed $\mathbf{z}$. \textbf{Right:} Diffusion process of original images}
\label{a:interpolation}
\end{figure}
